# Supplementary material for: openJiuwen: Beyond Static Harnesses for Long-Horizon Coding Agents
Source: arXiv:2608.27969 source file (2026-11-05)
Supplement: Supplementary file 1 [file appendix.tex]

\section{Additional material}
\label{app:extra}
% =============================================================================

Content placed after \verb+\appendix+ is lettered rather than numbered
(Appendix~\ref{app:extra}), and the axiom-style counters defined in
\verb+command.tex+ reset so they read \textit{A.1}, \textit{A.2}, and so on. Use
the appendix for proofs, extended tables, additional experiments, or verbatim
prompts that support --- but are not essential to --- the main text.
